# Supplementary material for: Microscopic coexistence of antiferromagnetic order and superconductivity in Ba$_{0.77}$K$_{0.23}$Fe$_{2}$As$_{2}$
Source: arXiv:1204.2434 source file (2012-11-06)
Supplement: Supplementary file 1 [file Supplemental_Material_86_180501.pdf]

Supplemental Materials for “Microscopic coexistence of antiferromagnetic order and superconductivity in  $\text{Ba}_{0.77}\text{K}_{0.23}\text{Fe}_2\text{As}_2$ ” by Z. Li *et al.*

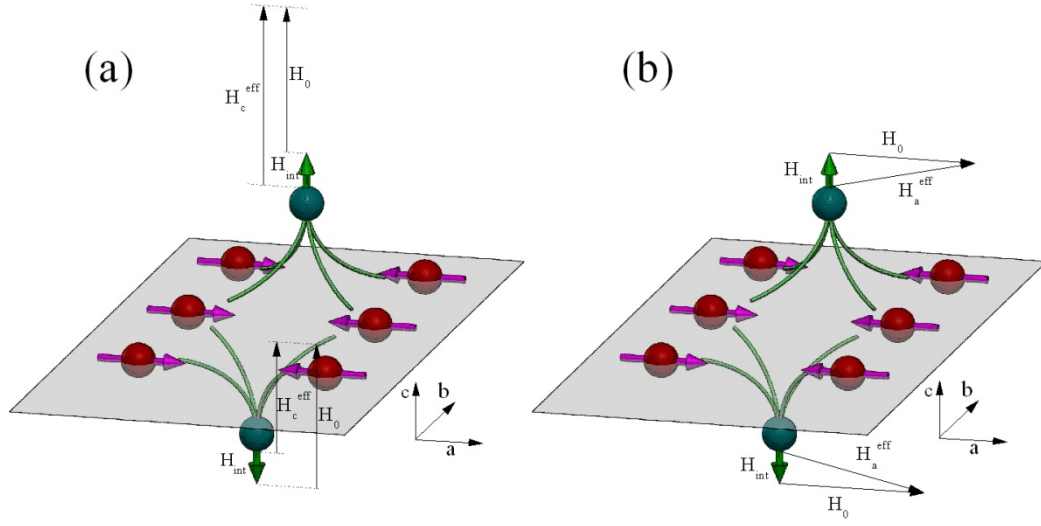

Fig. S1: The effective magnetic field ( $H^{\text{eff}}$ ) at the As-sites, with the external field ( $H_0$ ) applied along the  $c$ -axis (left) and along the  $a$ -axis (right), respectively.

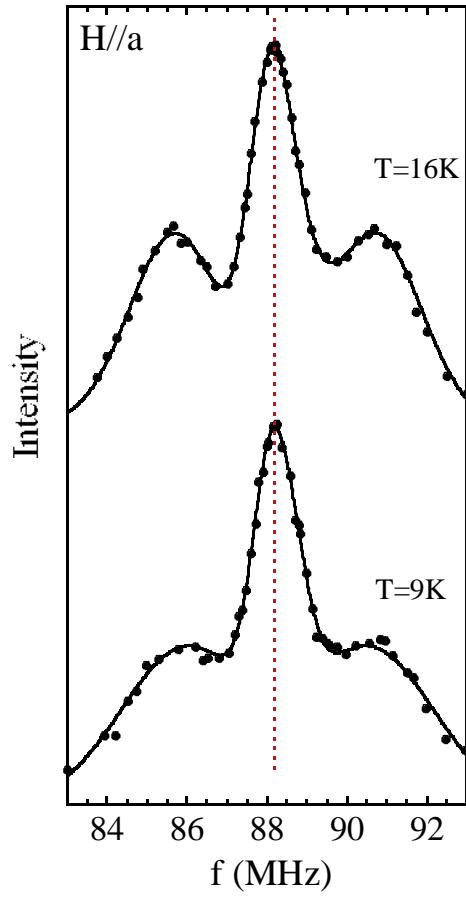

Fig. S2: The spectra for  $T=16\text{ K}$  (at  $T_c$ ) and  $T=9\text{ K}$  (below  $T_c$ ) with  $H//a$ .

Figure S2 shows the spectra for  $T=16\text{ K}$  (at  $T_c$ ) and  $T=9\text{ K}$  (below  $T_c$ ) with  $H//a$ . The dotted line is a guide to the eyes to show the position for the central peak.
